# Supplementary material for: Learning to Limit Data Collection via Scaling Laws: A Computational Interpretation for the Legal Principle of Data Minimization
Source: arXiv:2107.08096 source file (2022-06-13)
Supplement: Supplementary file 1 [file 98_appendix.tex]

% \documentclass[sigconf]{acmart}

% \usepackage{xr-hyper}
% \usepackage{hyperref}

% \makeatletter
% \newcommand*{\addFileDependency}[1]{% argument=file name and extension
%   \typeout{(#1)}
%   \@addtofilelist{#1}
%   \IfFileExists{#1}{}{\typeout{No file #1.}}
% }
% \makeatother

% \newcommand*{\myexternaldocument}[1]{%
%     \externaldocument{#1}%
%     \addFileDependency{#1.tex}%
%     \addFileDependency{#1.aux}%
% }

% \myexternaldocument{main} 

% \begin{document}
% \input{99_notation}
% \section{Experimental Details}

% We include relevant details to our experimentation below and provide code to reproduce all results.

% \subsection{Dataset Pre-Processing}
% \label{sec:data-pipeline} 
% For MovieLens-20M, we filter out users with fewer than 100 movies rated to produce a dataset of 51869 users and 26654 unique movies. MovieLens-L randomly samples 5000 users from this set and MovieLens-S samples 1000 users. For GoogleLocal, we filter out users with fewer than 150 ratings to produce a dataset of 1571 users and 275402 unique places. GoogleLocal-L randomly samples 1500 users from this set and GoogleLocal-S samples 500 users. Table 1 summarizes the dimensionality and sparsity of the resulting datasets.

% \subsection{Parameter Fitting}
% \label{sec:parameter-fitting} In line with past work, our method and each baseline is subject to the same parameter fitting approach: weighted non-linear least squares (NLSw). NLSw weights each sample by $( 1/\sqrt n)$, where $n$ is the sample size. This is done to account for the heteroscedastic relationship between performance  and dataset size. 

% \subsection{Implementation}\label{sec:implementation-details} We fit performance curves using the OLS implementation included in the Python statsmodels library \cite{seabold2010statsmodels} and the Levenberg-Marquardt algorithm via the least-squares implementation in the Python sklearn library \cite{scikit-learn}. All experiments were run on a 2.8 GHz Intel Core i7 processor with 16GB of available RAM on MacOS High Sierra.

% \subsection{Choice of thresholds}\label{sec:threshold-choice} We evaluate each method at three thresholds for the return on additional data: 5e-7, 2e-7, and 5e-8.  We select these thresholds because they translate to thresholds that are distributed over the data collection process (see Figure \ref{diminishing_returns_fig} to observe typical range of empirical returns for MovieLens-L and GoogleLocal-L). 

% \subsection{Implementation of Oracle} \label{sec:oracle-implementation} 

% To make our calculation of the slope using for the \emph{Oracle} baseline explicit, recall that we  generate $|\dmHistoricData|/\dmNumQueries$ subsamples over the course of data collection. To estimate the return in MSE at subsample $i$, we divide the difference in empirical performance at subsample $i-2$ and subsample $i+2$ by their difference in sample sizes, or $4\dmNumQueries$. This produces an approximation of the true return that is sufficiently smooth; we experiment with a different smoothing procedure (estimation via subsample $i-1$ and subsample $i+1$) later in the supplemental material.


% \section{Supporting Figures}
% \subsection{Minimization on Returns: Consistent Results}
% \label{sec:other-datasets}

%  We plot consistent results in Figure \ref{supplemental_diminishing_returns_fig}. These results align with those  discussed in the body of the paper; while our method appears noisier, it reflects the noise of the empirically derived return in additional data. If one were to minimize with respect to a less noisy metric than performance given additional examples, this curve may look smoother. This presents yet another tradeoff between the baselines and the proposed method: while our method produces stopping points most accurate to the empirical return on additional data, the baselines offer a ``smoother" decision rule.

% % \subsection{Alternate Approximation of Oracle Slope/Return on Data} We offer results with respect to a slightly different approximation of the true return (smoothed over two samples, rather than four) in Table \ref{diminishing_returns_table_different_approx}. The proposed data collection method  stops data collection at the point closest to the empirically derived stopping point, given an alternate empirical derivation of the true slope.

% \begin{figure*}[t!]
%     \centering
%     \includegraphics[width=1\textwidth]{LaTeX/figs/supplemental_diminishing_returns_fig_three_stages.png}
%     \vspace{-0.7cm}
%     \caption{\textbf{Evaluation of performance curves over the course of data collection.} We plot the diminishing returns results for MovieLens-S and GoogleLocal-S visually here. Note that the margin with which we outperform baselines is smaller in the case of MovieLens-S; this is due to the smaller diminishing returns region, which can be seen in Figure \ref{stability_performance_curve}.}
%     \label{supplemental_diminishing_returns_fig}
%     \vspace{-0.2cm}
% \end{figure*}

% % \input{98_01_alternate_slope_table}

% \subsection{Comparisons to Other Curve Models}
% \label{sec:other-baselines}

% \subsubsection{Ablation of Stages in Piecewise Power Law} 
% \label{sec:two-stage-power-law} 
% FIDO uses a piecewise power law technique that consists of three power laws, or one for each stage of data collection outlined by \cite{hestness1712deep}. In this section, we provide an ablation study of the necessity of each stage by testing FIDO with one power law, two power laws, and three power laws (Table \ref{diminishing_returns_ablation_table}). In short, the use of three power laws produces more accurate stopping criteria \emph{on average}, but the stopping criteria are not significantly different from modeling two stages. This is because the "small data region" is negligibly small in most cases, and performance is not affected by modeling the small data region and the power law region as one power law.

% \input{98_02_stage_ablations}

% \subsubsection{Nonparametric Regression}
% \label{sec:nonparametric-regression}
% Each of the baselines considered are parametric approximations of the relationship between dataset size and performance. Past work in learning curve estimation considers the value of nonparametric approaches. Here, we explore the value of such an approach and find that the estimated performance curves are much noisier than those produced by parametric curve models. Table \ref{nonparam_table} shows that FIDO achieves more accurate stopping criteria across datasets and thresholds, by a large margin.

% \input{98_03_nonparam_comparison}

% \subsection{Performance Curves for GoogleLocal-S and MovieLens-S}
% \label{sec:random-perf-curves}

% We include the performance curves for each dataset considered in this work in Figure \ref{fig:all_performance_curves}. We include the performance curves for MovieLens-L and GoogleLocal-L, as shown in Figure \ref{perf_curves} for ease of comparison.


% \subsection{Performance Curves for Active vs. Random Feature Acquisition}
% \label{sec:afa-perf-curves}

% We include the true performance curve using \emph{Stability} as a feature acquisition algorithm in Figure \ref{stability_performance_curve}. Note the noise introduced over runs compared to the performance curves produced by random feature acquisition (Figure \ref{perf_curves}).

% \subsection{Illustrative Performance Curve Fits}
% \label{sec:pc-fit-illustrations}
% We measure the quality of the performance curve fit via metrics relevant to our data minimization objectives (extrapolations and slope estimation) in the body of the paper and support these results with a visualization of performance curve fits (Figure \ref{illustrative}). We plot each method's performance curve fit halfway through data collection from GoogeLocal-L. Examining the predicted performance curve (orange) for each baseline, we can see that it departs from the true performance curve most towards the end of data collection, due to differences in modeling the stage of diminishing returns. 

% \section{Alternate Data Minimization Objective: Minimization by Relative Performance}
% \label{sec:alternate-dm-objective}

% In the body of the paper, we consider one data minimization objective: minimization based on the return of additional data. FIDO is flexible to other performance-based objectives as well. In this section, we explore one such objective: minimization based on the \emph{relative performance}, which stops data collection based on a percentage of the model's performance given infinite data.

% \paragraph{Definition} Minimization in reference to a relative performance rather than an absolute performance may be preferable because it is difficult to identify a good goal performance without understanding (1) model performance in the absence of additional data and (2) model performance in the presence of all available data. Parameter $\dmGainThreshold$ represents the goal \emph{fraction} of performance gain and dictates when the stopping criterion should be enforced. The parameter can be set globally, or individually for each user. The fraction of performance gain is a relative performance metric, scaled between the model performance given no additional data and model performance given all available data. Under the considered scenario, the data minimization task is to collect the minimum number $\dmBudget$ of user-feature-value triples from queryable set $\dmPool$ such that the fraction of performance gain achieved equals at least $\dmGainThreshold \in [0, 1]$: 

% \begin{equation}
% \frac{\dmPerformanceStarting - \dmPerformanceTreatment}{\dmPerformanceStarting-\dmPerformanceTarget} \geq \dmGainThreshold
%     % \frac{\sigma(M, I) - \sigma(M, I + H(P, n))}{\sigma(M, I) - \sigma(M, I + P)} \geq g,
% \end{equation}

% \paragraph{Results}  Minimization by relative performance requires approximating the percentage of performance gain using the performance curve learned in Step 2 and ceasing data collection once the predicted performance gain exceeds user-specified goal $g$. The proposed method ceases data collection at a point closest to the goal percentage compared to baselines and its performance offers insight into the reliability of relative-performance-based stopping criteria.

% We evaluate each stopping criterion across multiple datasets and goal fractions of performance $\dmGainThreshold \in [.5, .6, .7,.8, .9]$. The plots show that lower goals are more difficult to adhere to, producing larger gaps between the true performances accomplished by each method and the goal performance (plotted in red). While the method performs significantly better than baselines in some cases (particularly for higher goal percentages on GoogleLocal-L), we cannot confidently conclude that the proposed method produces a significantly better stopping criteria across datasets. This suggests the selection of the appropriate performance curve model may depend both on the dataset and the data minimization objective.

% It is worth noting that most methods, save for \emph{3P-PL-Exp}, collect more data than is necessary for the goal performance, producing true performance gains that exceed $\dmGainThreshold$. This is a direct result of each method’s underestimation of the error on the test set given the queryable set $\dmPool$, as discussed in earlier sections. Minimized data collection must be conscious of this behavior, because such algorithms are liable to collect too much data for a given goal.

% \begin{figure*}[t!]
%     \centering
%     \includegraphics[width=\textwidth]{LaTeX/figs/stopping_criteria_three_stages.png}
%     \caption{\textbf{Performance on Relative Performance Minimization} The proposed method (green) lands closest to the goal percentage of relative performance on average, compared to existing methods. While the piecewise power law produces a power law curve that is significantly more accurate than others in \textit{forecasting} performance, the estimates of relative performance remain comparable to baselines.}
%     \label{stopping_criteria}
% \end{figure*}

% \begin{figure*}[t!]
%     \centering
%     \includegraphics[width=\textwidth]{LaTeX/figs/all_perf_curves_line.png}
%     \caption{\textbf{Performance Curves given Random Feature Acquisition} Each graph represents the improvement in performance over the course of data collection. Note the smaller diminishing returns region for MovieLens-S.}
%     \label{fig:all_performance_curves}
% \end{figure*}

% \begin{figure*}[t!]
%     \centering
%     \includegraphics[width=\textwidth]{./LaTeX/figs/stability_performance_curves.png}
%     \caption{Performance curves using AFA method \emph{Stability}. Each line represents an individual split of the dataset.}
%     \label{stability_performance_curve}
% \end{figure*}

% \begin{figure}[t!]
%     \centering
%     \includegraphics[width=.5\columnwidth]{LaTeX/figs/illustrative_fits.png}
%     \caption{Performance curve fits halfway through data collection for our method and the 4 baselines considered. The black dotted line denotes the amount of data provided to each performance curve fit---note that \emph{2P-Power-Law-Initial} sees no more than the initial dataset. }
%     \label{illustrative}
% \end{figure}

% \label{appendix:related_work}
% \section{Additional Related Work}

% \subsection{Active Feature Acquisition (AFA).}
% AFA concerns the intelligent collection of feature-values given a fixed budget. There are several well-known AFA techniques: (i) using matrix completion with the assumption of low rank \cite{doi:10.1137/1.9781611974973.30, pmlr-v54-bhargava17a, huang2018active} (ii)  estimating the expected accuracy improvement for tasks such as clustering or classification \cite{Vu_intelligentinformation, 10.1109/ICDM.2005.23} (iii) applying techniques to address ice-start \cite{gong2019icebreaker} and cold-start problems \cite{10.1145/564376.564421} and (iv) using variational techniques to approximate the posterior distribution \cite{10.1145/2487575.2487627}. The performance of AFA is often evaluated based on a fixed budget. FIDO lies adjacent to this area in that the framework aims to learn a performance-based budget \textit{given} a feature acquisition algorithm. 


% \subsection{Sample Complexity.} Sample complexity corresponds to the number of samples required for a learning algorithm to achieve an error rate of $\epsilon$ with a probability of $(1 - \delta)$. Literature on sample complexity takes a theoretical approach to the central task of our work: tying data collection to model performance. Earlier work quantifies sample complexity assuming random sample acquisition \cite{ehrenfeucht1989general}, while more recent work studies sample complexity for active learning methods \cite{yan2019label, balcan2010true} and recommendation systems \cite{heckel2017sample}. \citet{hestness1712deep} note the gap between theoretical guarantees and empirical trends for performance curves and highlight this as an area for future work.

% \bibliographystyle{unsrt}
% \bibliography{main}

% \end{document}
